# Supplementary material for: Variable Selection for Comparing High-dimensional Time-Series Data
Source: arXiv:2412.06870 source file (2024-12-09)
Supplement: Supplementary file 1 [file demo-sumo-most.tex]

\section{SUMO Monaco Scenario generation}

\label{sec:app-SUMO-details}

\subsection{Scenario Description in Detail}

The road blocking commences at the time step of $17,000$ and continues until the end of the scenario.

\subsection{Data Representation}
\label{sec:sumo-description-data-collection}

A simulation collects metrics per edge which is a segmented area of a road.
For simplicity and consistency, we call "edge" as "road" in this paper.
A road records these three metrics: \emph{traffic count, waiting time, density}\footnote{We use SUMO's function of recording metrics per road. Please refer to the following documentation for the definitions of metrics. \url{https://sumo.dlr.de/docs/Simulation/Output/Lane-_or_Edge-based_Traffic_Measures.html}}.
There are $4,404$ roads in a study area.

From a simulation, given a set of roads $R = \{r_1, ..., r_{4404}\}$ and simulation time steps $T'  = \{t'_{1}, ..., t'_{{50400}}\}$, each road $r$ aggregates the observation values during 10 time steps.
Hence, the aggregated time steps is $T = \{t_1, ...., t_{5040}\}$ where each $t$ is an aggregation of observed values during 10 steps.
Let $V^r_{t'}$ a set of vehicles existing on the road $r$ at a time steps $t'$.
The traffic count is the number of vehicles located on a road $r$ during the aggregated time steps $t$.

$${\rm Count}_{{t}}^{r} = \sum_{t'=10(t-1)+1}^{10(t-1) + 10} {\rm Count}(V^r_{t'}),$$
where $\text{Count}(V^r_{t'}) \in \mathbb{R}$.
Note that the traffic count does not necessarily have to be an integer value, but can be a float value since a vehicle may exist on a boundary of a road $r$ and the vehicle is counted by a ratio of the vehicle's body located on the road $r$.

The waiting time measures the sum of time steps that vehicles $V^r_{t'}$ are with the status of speed=0.
The edge waiting time is defined as follows,

$$\rm{Waiting Time}_{{t}}^{r} = \sum_{t'=10(t-1)+1}^{10(t-1) + 10} \sum_{v=1}^{|V^r_{t'}|} {\rm Waiting\ Time}_{t'}^{v},$$
where ${\rm Waiting\ Time}_{t'}^{v} \in \mathbb{R}$ is the time that a vehicle is in the status of speed=0. 

The density is a metric to measure the occupied area by vehicles at a road $r$;
i.e. the edge density increases as the number of vehicles increases at a road $r$.

$$\rm{Density}_{{t}}^{r} = \sum_{t'=10(t-1)+1}^{10(t-1) + 10} \frac{Count(V^r_{t'})}{KM_r},$$ 
where ${\rm KM}_r$ is the length of the road $r$, which is in kilometre.

We adopt these three metrics by the following assumptions;
when roads are blocked, more vehicles may select a specific route.
Due to this high traffic volume, a road would have more density and therefore traffic jams would occur.
As a consequence, vehicles have to wait longer on a specific road and require longer travel time.

\textcolor{red}{deleteing the waiting time}.
The top two figures of Figure~\ref{fig:demonstration-most-simple-aggregation-and-pval} describe summaries of the ``Traffic count'' and ``Waiting time.'' 
In each figure at each step $t$, the depicted are the mean and standard deviation of $x_{t,1}, \dots,x_{t,d}$ (blue) and those of $y_{t,1}, \dots,y_{t,d}$. 
There are some discrepancies between $X$ and $Y$, particularly for the Waiting Time statistics. \\

\begin{figure}[h]
    \centering
    \includegraphics[width=.47\textwidth]{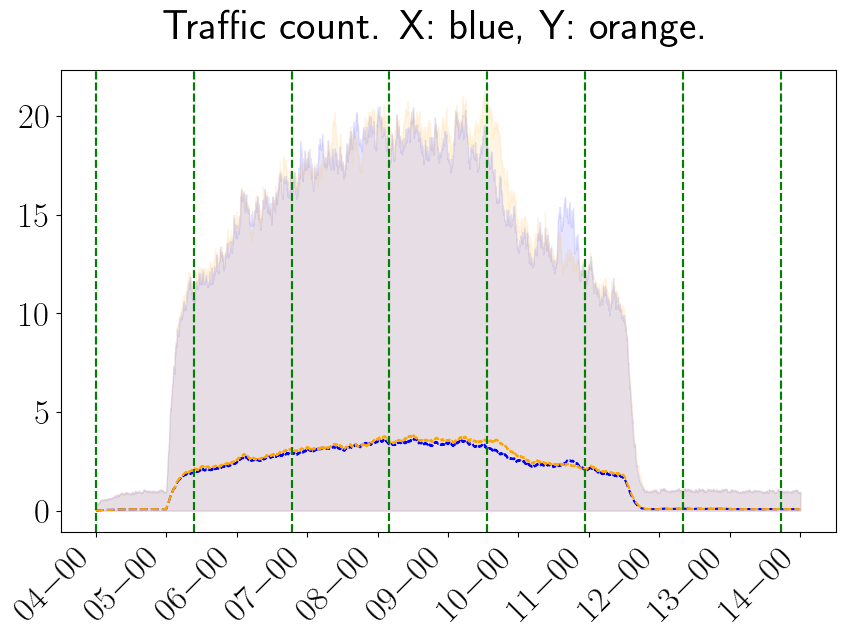} \ \
    \includegraphics[width=.47\textwidth]{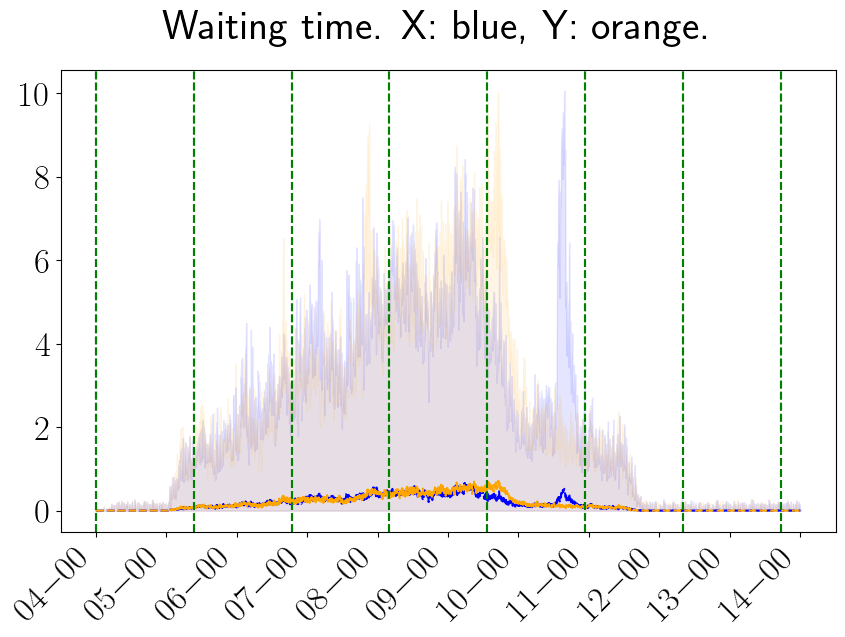} 
    \caption{
        Summaries of the statistics, Traffic Count (left) and Waiting Time (right), for data representation in Section~\ref{sec:sumo-description-data-collection}.
        The solid lines are the average values over different road segments at each time step, and the shaded areas are the standard deviations.
        The blue indicates data $X$ from the original {\tt MoST} scenario, and the red indicates data $Y$ from the modified scenario.
        The green vertical dashed lines are the time-splitting points. 
    }
    \label{fig:summary-data-traffic}
\end{figure}

\subsection{Analysis by Density metric}
\label{sec:sumo-description-variable-selection}

In Section~\ref{sec:demonstration-most}, we demonstrate the model comparisons with metrics of the traffic count and waiting time.
In this section, we demonstrate the model comparisons with the density metric.
The definition of the density metric is in Section~\ref{sec:sumo-description-data-collection}.
In the same manner as Section~\ref{sec:demonstration-most}, we collect observations of the density metric.
Figure~\ref{fig:demonstration-most-simple-aggregation-density}~(Left) visualises the aggregation of all roads by the average and the standard deviation,
and Figure~\ref{fig:demonstration-most-simple-aggregation-density}~(Right) shows the p-value sequence of the permutation test by three variable selection methods.
Among three variable selection methods, the \codeName{wasserstein-base} often accepts $H_0$ while the other two MMD-based variable selections reject $H_0$.
The \codeName{wasserstein-base} rejects $H_0$ at the bucket $\bucketIndex{5}$.
That seems to be because the difference in the average values between $X, Y$ are apparent.
Paying attention to differences in the standard deviations between $X, Y$ in Figure~\ref{fig:demonstration-most-simple-aggregation-density}~(Left),
it sounds like differences in the standard deviations.
Moreover, it sounds natural that distributions of the density metric would be dissimilar between $X, Y$ since vehicles in the simulation $Q$ reroute to the Monaco centre instead of travelling via the A8.
As a result of this rerouting, at least, the density of the A8 and the roads at the Monaco centre would be significantly different.
Considering these factors, we would conclude that the \codeName{wasserstein-base} results in accepting $H_0$ because it selects too many variables than necessary.
This phenomenon of selecting too many variables would be due to a drawback of the \codeName{wasserstein-base} that it does not consider interactions between variables.
On the other hand, the MMD-based methods select variables of having responsibilities of rejecting $H_0$, therefore, the two successfully reject $H_0$.

\begin{figure}[t]
    \centering
    \includegraphics[scale=0.3]{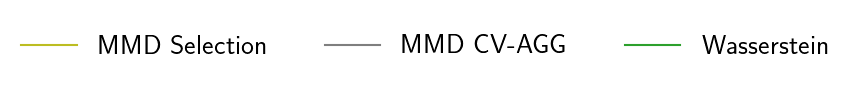} \hfill
    \\
    \includegraphics[width=.44\textwidth]{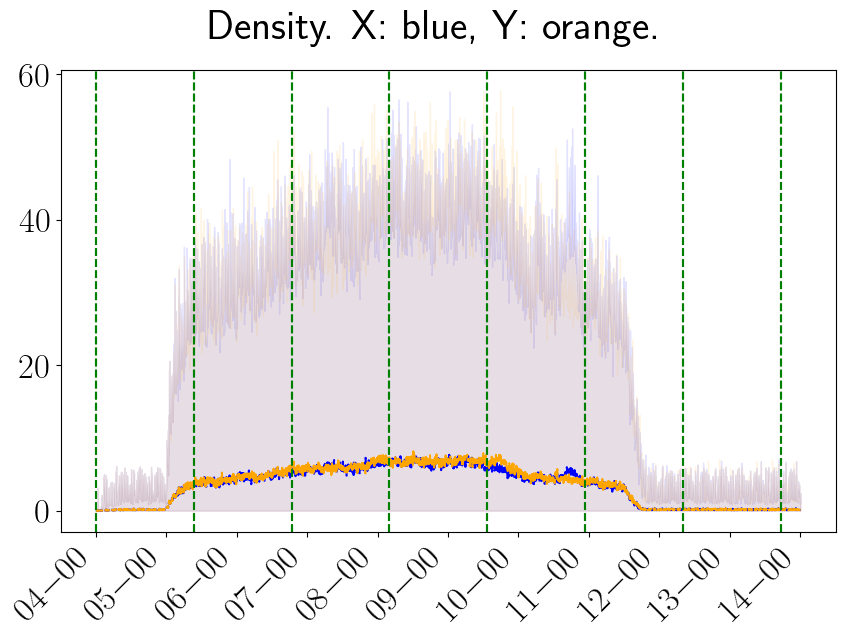} \hfill
    \includegraphics[width=.44\textwidth]{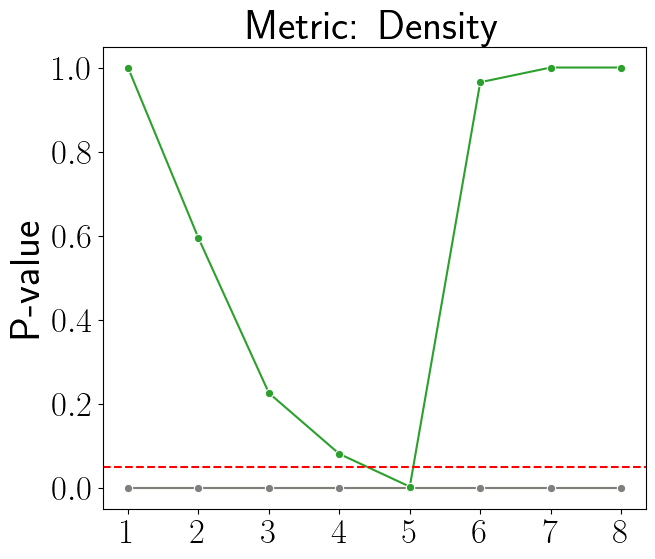} \hfill
    \caption{
        (Left) the average and standard deviation over all roads with the density metric.
        (Right) the p-value sequence of the permutation test by three variable selection methods.
        More description is in Section~\ref{sec:sumo-description-variable-selection}.
    }
    \label{fig:demonstration-most-simple-aggregation-density}
\end{figure}

\subsection{Naive Approach: a naive L1 distance v.s. variable selection methods}
\label{sec:sumo-description-simple-aggregation}

Figures~\ref{fig:sumo-heatmaps-traffic-count}, \ref{fig:sumo-heatmaps-waiting-time} and \ref{fig:sumo-heatmaps-density} are comparisons of the averaged L1 distance, \codeName{Wasserstein-based}, \codeName{MMD Selection} and \codeName{MMD-CV} variable selection methods.
The definition of the average L1 distance is the same as Equation~\ref{eq:average-l1-distance}.
The heatmaps are generated by the average of the absolute differences per 500 time steps.
The three heatmaps of the variable selection method do not show colour bars when the p-value $>0.05$ at the bucket $\bucket$, i.e. a bar is coloured with all black.

Comparing the heatmaps of the averaged L1 distance and the variable selection methods, the variable selection methods successfully discover variables that the averaged L1 distance does not.
For example, the variable selection methods discover the road $r=1474$ in the traffic count metric, the road $r=1340$ in the edge density metric, and the road $r=1474$ in the edge waiting time metric.
These tendencies are the same for the metrics of the density and waiting time.
By this comparison, it is apparent that the variable selection methods are useful for discovering the major influences on the traffic flow by the perturbation in the study area.
These apparent differences are natural because the averaged L1 distance is susceptible to the observed values, for example, the observed values of the traffic count.

\begin{figure}[h]
    \begin{subfigure}{0.45\textwidth}
        \centering
        \includegraphics[scale=0.35]{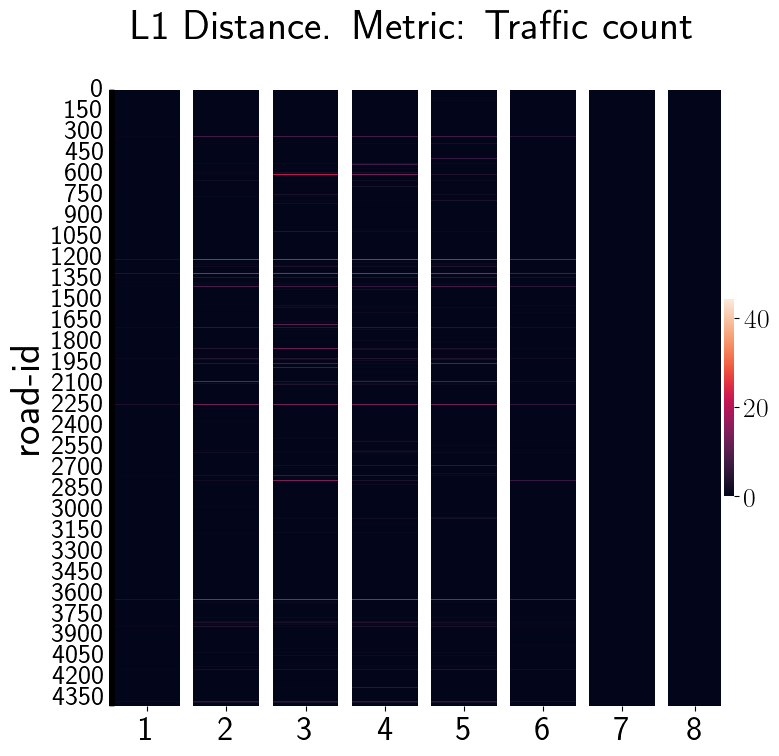} 
        \caption{Averaged L1 distance}
    \end{subfigure}
    \hfill
    \begin{subfigure}{0.45\textwidth}
        \centering
        \includegraphics[scale=0.35]{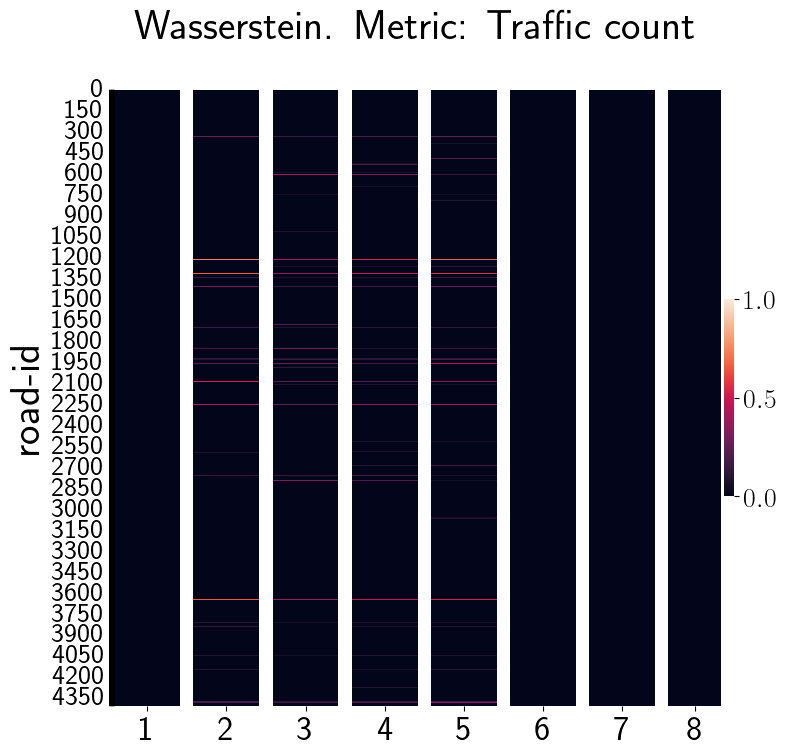} 
        \caption{\codeName{Wasserstein-based}}
    \end{subfigure}

    \begin{subfigure}{0.45\textwidth}
        \centering
        \includegraphics[scale=0.35]{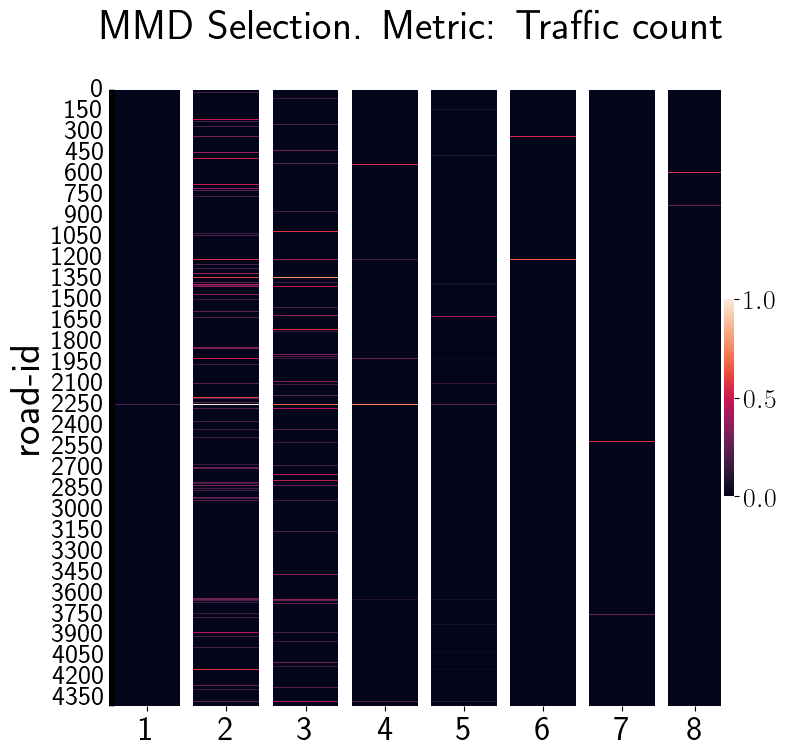} 
        \caption{\codeName{MMD Selection}}
    \end{subfigure}
    \hfill
    \begin{subfigure}{0.45\textwidth}
        \centering
        \includegraphics[scale=0.35]{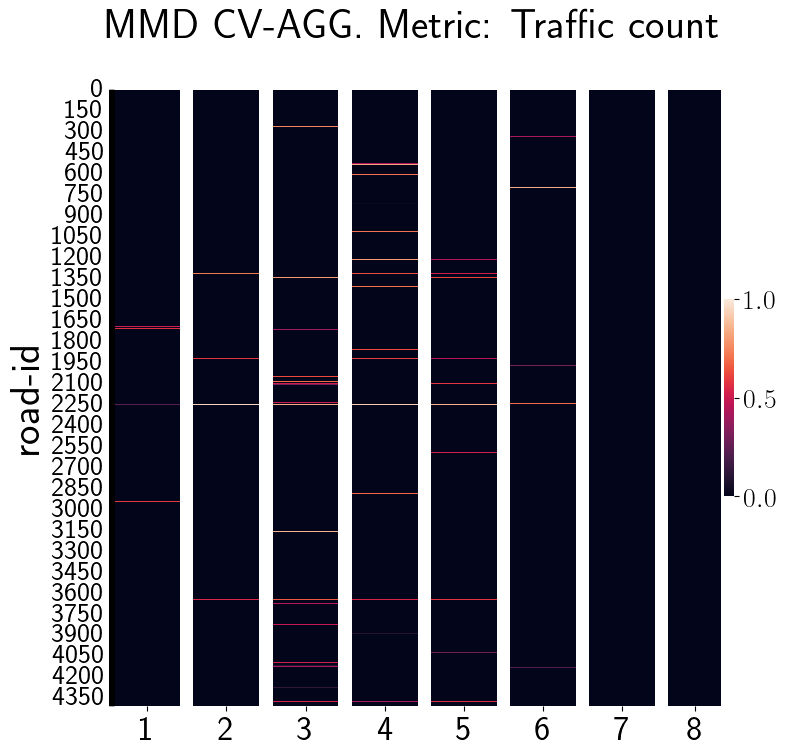} 
        \caption{\codeName{MMD CV}}
    \end{subfigure}
    \caption{
        Comparisons of the averaged L1 distance, \codeName{Wasserstein-based}, \codeName{MMD Selection} and \codeName{MMD-CV} variable selection methods.
        The study metric is \codeName{traffic count}.
    }
    \label{fig:sumo-heatmaps-traffic-count}
\end{figure}

\begin{figure}[h]
    \begin{subfigure}{0.45\textwidth}
        \centering
        \includegraphics[scale=0.35]{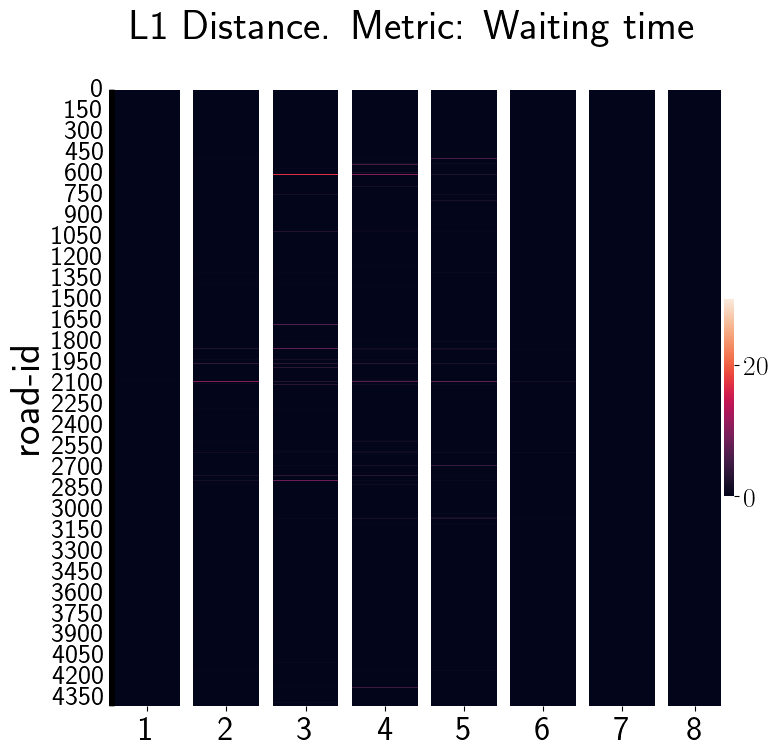} 
        \caption{Averaged L1 distance}
    \end{subfigure}
    \hfill
    \begin{subfigure}{0.45\textwidth}
        \centering
        \includegraphics[scale=0.35]{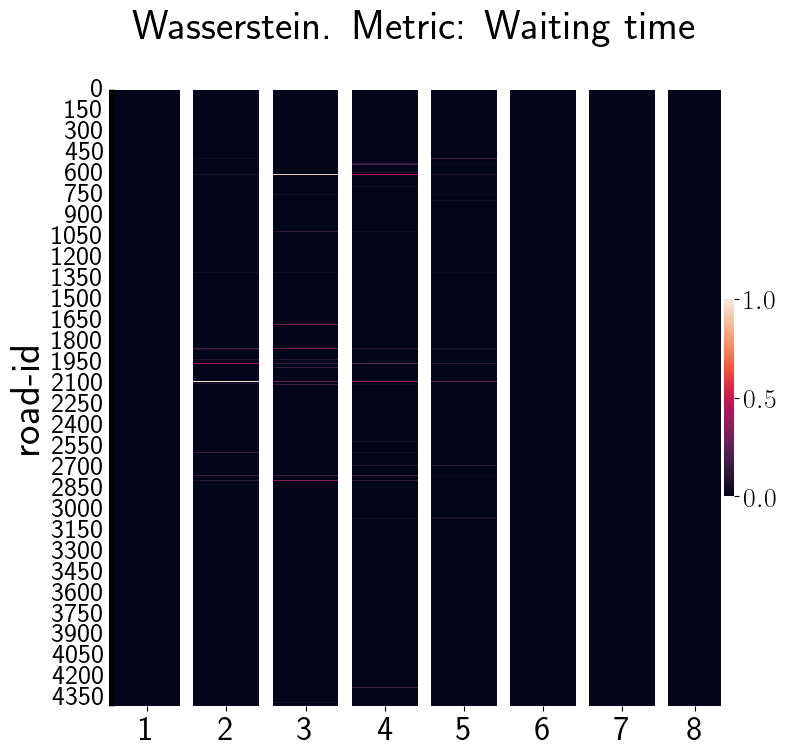} 
        \caption{\codeName{Wasserstein-based}}
    \end{subfigure}

    \begin{subfigure}{0.45\textwidth}
        \centering
        \includegraphics[scale=0.35]{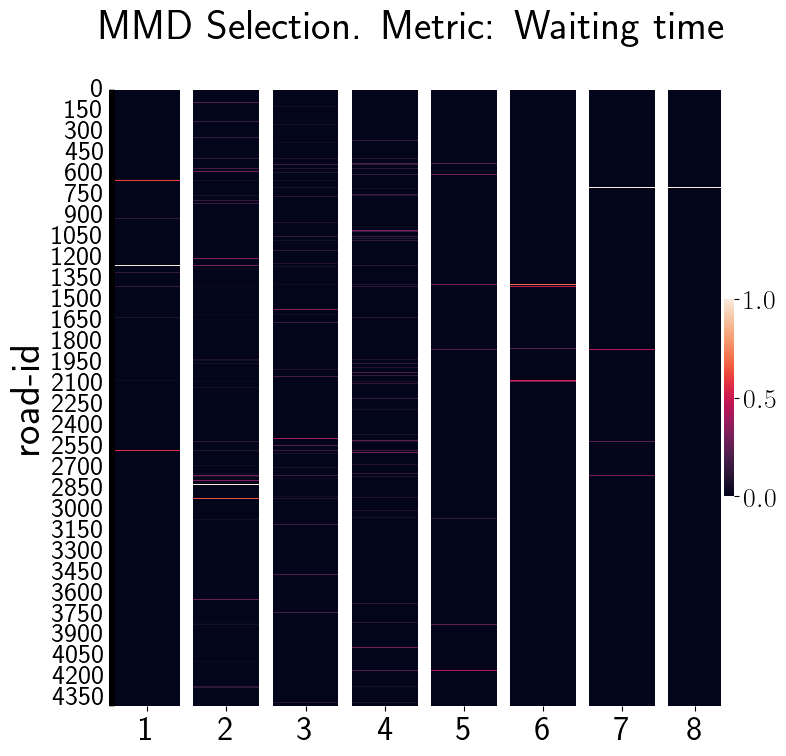} 
        \caption{\codeName{MMD Selection}}
    \end{subfigure}
    \hfill
    \begin{subfigure}{0.45\textwidth}
        \centering
        \includegraphics[scale=0.35]{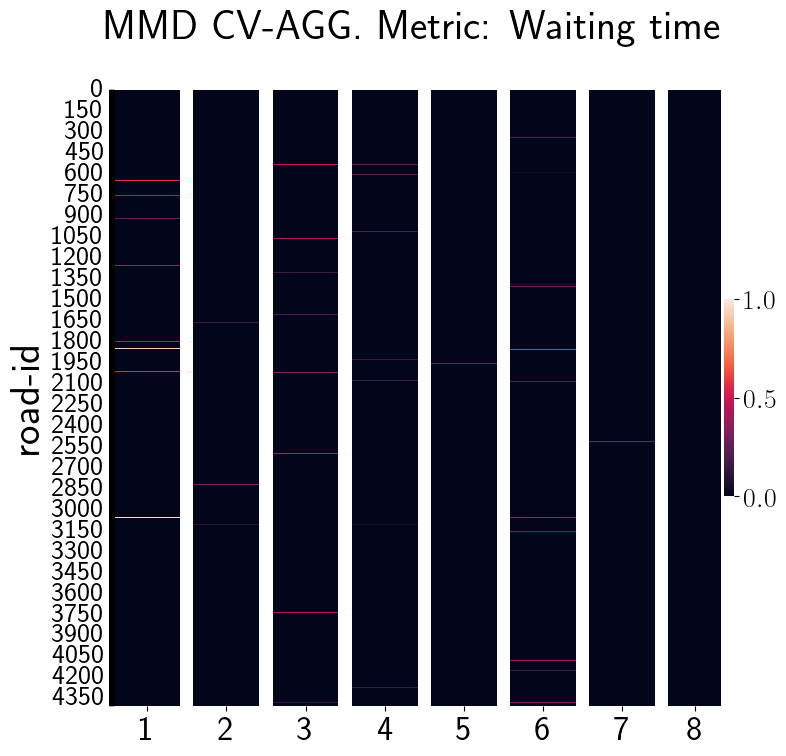} 
        \caption{\codeName{MMD CV}}
    \end{subfigure}
    \caption{
        Comparisons of the averaged L1 distance, \codeName{Wasserstein-based}, \codeName{MMD Selection} and \codeName{MMD-CV} variable selection methods.
        The study metric is \codeName{waiting time}.
        }
    \label{fig:sumo-heatmaps-waiting-time}
\end{figure}

\begin{figure}[h]
    \begin{subfigure}{0.45\textwidth}
        \centering
        \includegraphics[scale=0.35]{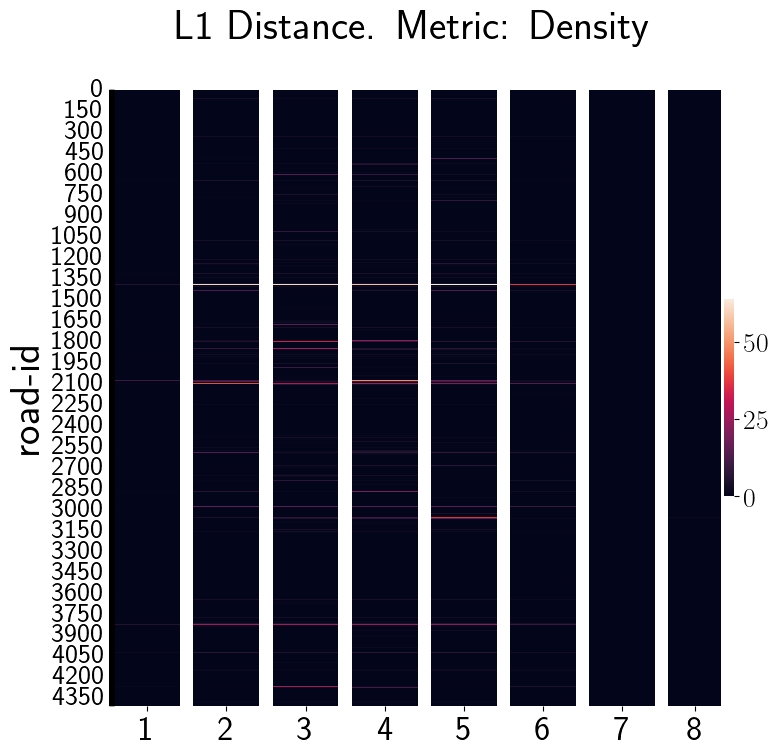} 
        \caption{Averaged L1 distance}
    \end{subfigure}
    \hfill
    \begin{subfigure}{0.45\textwidth}
        \centering
        \includegraphics[scale=0.35]{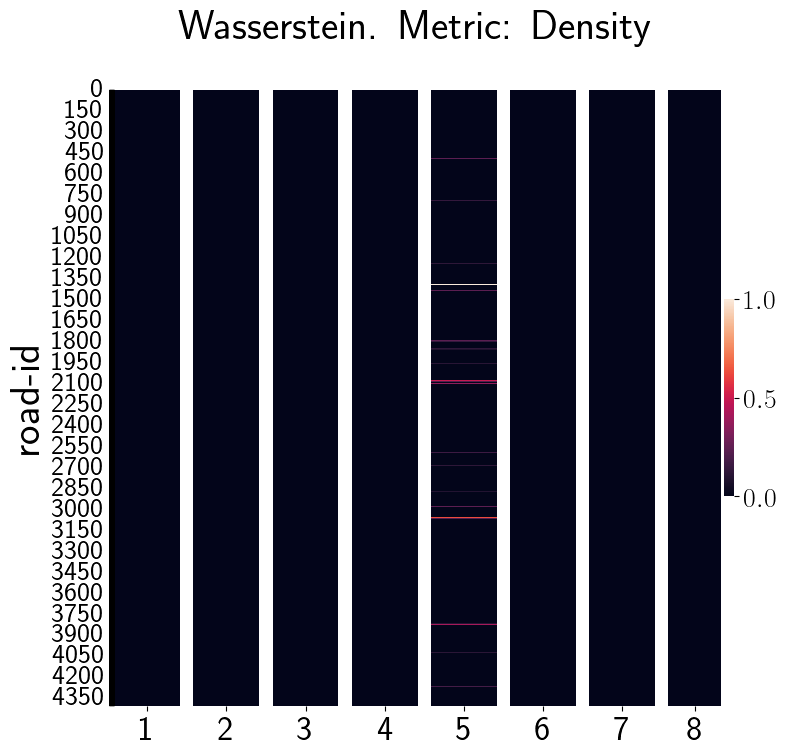} 
        \caption{\codeName{Wasserstein-based}}
    \end{subfigure}

    \begin{subfigure}{0.45\textwidth}
        \centering
        \includegraphics[scale=0.35]{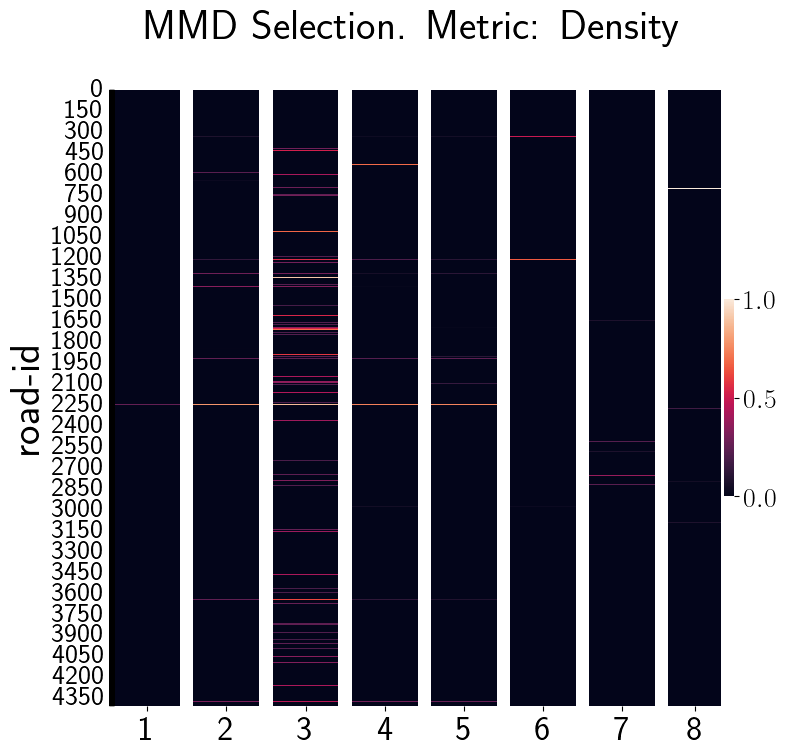} 
        \caption{\codeName{MMD Selection}}
    \end{subfigure}
    \hfill
    \begin{subfigure}{0.45\textwidth}
        \centering
        \includegraphics[scale=0.35]{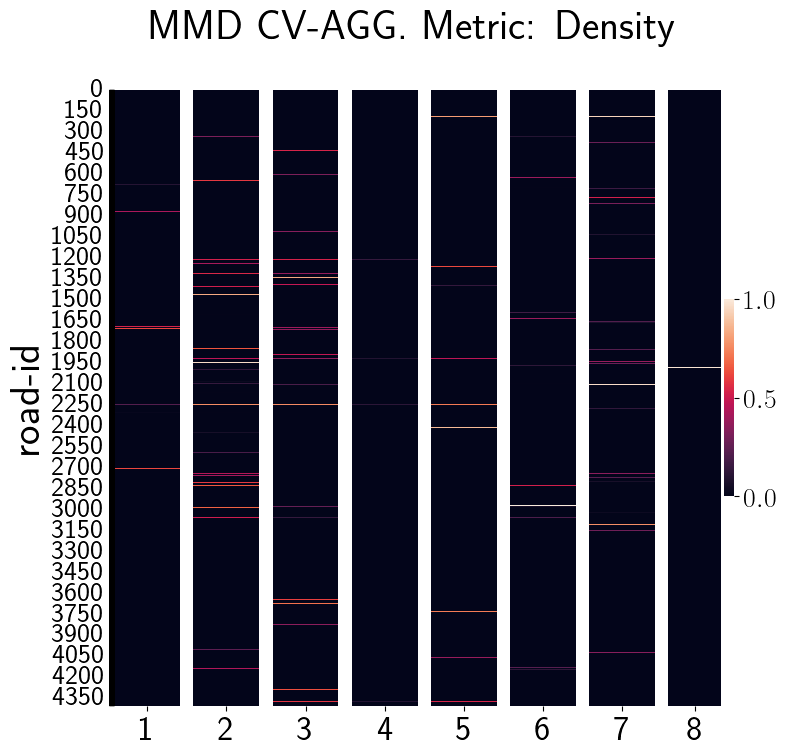} 
        \caption{\codeName{MMD CV}}
    \end{subfigure}
    \caption{
        Comparisons of the averaged L1 distance, \codeName{Wasserstein-based}, \codeName{MMD Selection} and \codeName{MMD-CV} variable selection methods.
        The study metric is \codeName{density}.
        }
    \label{fig:sumo-heatmaps-density}
\end{figure}
