# Supplementary material for: Variable Selection for Comparing High-dimensional Time-Series Data
Source: arXiv:2412.06870 source file (2024-12-09)
Supplement: Supplementary file 2 [file variable-selection-trajectory.tex]

\section{Variable Selection for trajectory data}
\label{sec:appendix-variable-selection-trajectory}

The demonstration cases illustrate situations where both the simulation outputs and their counterparts consist of observation data from a set of sensor records.
However, there are use-cases in which one is interested in the differences of the trajectory data or directions of the trajectory data of simulation agents.
The trajectory data is, for example, the geo-coordinates of simulation agents.
The variable selection on the trajectory data is useful when one is interested in discrepancies of the trajectory data or directions of the trajectory data.

Let $A \in \mathbb{N}$ be the number of simulation agents, $\TimeN$ be the number of time steps, and $C \in \mathbb{N}$ be a set of geo-coordinates, such as two or three-dimensional rectangular coordinate system by $(x, y)$ when $C=2$ or $(x, y, z)$ when $C=3$.
A trajectory data consists of $\mathbb{R}^{A \times \TimeN \times C}$.
Since we are interested in directions of trajectories, two time series $X, Y$ are $X = (x_1,\threeDots,x_T), Y = (y_1,\threeDots,y_T), x, y \in \mathbb{R}^{A \times (\TimeN-1) \times C}$.
The number of time steps is $\TimeN - 1$ since we consider differences in trajectories (direction) between time steps

In the time-slicing algorithm in Algorithm~\ref{alg:time-slicing-variable-selection}, we split the set of time steps into $\TotalBucketSize$ buckets.
In each bucket $\bucket$, the algorithm sets an interval $\bucketIndex{\bucket}$ of time steps per bucket $\bucket$ and randomly splits $\IntervalIndex{\bucket}$ into $\IntervalIndexTrain{\bucket}, \IntervalIndexTest{\bucket}$.
Following $\IntervalIndexTrain{\bucket}, \IntervalIndexTest{\bucket}$, we collect a set of samples $\sampleSetTrain{\datasetX}_{\bucket} = \{x_i | i \in \IntervalIndexTrain{\bucket} \}, \sampleSetTrain{\datasetY}_{\bucket} = \{y_i | i \in \IntervalIndexTrain{\bucket} \}$ for training and $\sampleSetTest{\datasetX_{\bucket}} =\{x_i | i \in \IntervalIndexTest{\bucket} \}, \sampleSetTest{\datasetY_{\bucket}} =\{y_i | i \in \IntervalIndexTest{\bucket} \}$ for testing, 
where $x, y$ consists of $\mathbb{R}^{A \times C}$ instead of $\mathbb{R}^{D}$ in the original algorithm.
The selected variables $S$ consist of variables of simulation agents $S \subset \{1,\threeDots,A\}$.

\subsection{Variable Selection for Trajectory Data}

The variable selection algorithm requires handling the trajectory data $\mathbb{R}^{A \times C}$.
Due to the implementation reasons, we introduce MMD-based variable selection and Wasserstein-based variable selection that we discuss in Section~\ref{sec:proposal-variable-selection}.
Both variable selection algorithms compute a weight term a weight term $w \in \mathbb{R}^{A}$. 
We denote weights for $i$-th simulation agent as $w_{i}$.
We show demonstrations of variable selection for the trajectory data using the particle simulation dataset in Appendix~\ref{sec:demonstration-particle-variable-selection-trajectory}.

\subsubsection{MMD-based Variable Selection for Trajectory Data}

The MMD-based variable selection employs a Gaussian kernel with an L2 distance function that is able to handle the two or three-rectangular coordinate system.
The Gaussian kernel is,

\begin{equation}
    k(x, y) = exp \left( - \frac{1}{A} \sum\limits_{i=1}^{A} \frac{ w_{i}^2 \sum\limits_{j=1}^{C} || x_{i}^{(j)} - y_{i}^{(j)} ||}{ \gamma^2_d } \right),
\end{equation}
where $w$ is ARD weights to be optimised by MMD optimisation at Equation~\ref{eq:mmd-optimisation-problem},
$x_{i}^{(j)}, y_{i}^{(j)}$ denote $i$-th simulation agent at $j$-th geo-coordinate, 
and $\gamma^2 \in \mathbb{R}^{A}$ is the length scale that we compute by the dimension-wise medial heuristic in our previous work~\citep{mitsuzawa-2023}.

\subsubsection{Wasserstein-based for Trajectory Data}

The wasserstein-based variable selection for the trajectory data employs a \emph{Sliced Wasserstein} distance~\citep{bonneel-2015} instead of a \emph{Wasserstein} distance.
The sliced wasserstein distance computes a distance per simulation agent, $\mathbb{R}^{C} \times \mathbb{R}^{C} \rightarrow \mathbb{R}$.
A weight for $i$-th simulation agent is 

\begin{equation}
    w_{i} = {\rm Sliced\ Wasserstein}(\datasetX^{i}, \datasetY^{i}),
\end{equation}
where $\datasetX^{i}, \datasetY^{i}$ are sample sets of $i$-th simulation agent $\datasetX^{i} = \{ x^i_j | j \in \Interval \}$, $\datasetY^{i} = \{ y^i_j | j \in \Interval \}, x^i_j, y^i_j \in \mathbb{R}^{C}$ having lengths of the bucket interval $\Interval$.

We use the implementation from Python POT package\footnote{\url{https://pythonot.github.io/all.html}}.
Since the sliced Wasserstein distance requires a hyperparameter of the number of random projections.
We select this hyperparameter where the the variance of five times sliced wasserstein computation is the smallest when we compute sliced wasserstein distances of which random projections per 10 steps from $[50, 500]$.
