# Supplementary material for: Variable Selection for Comparing High-dimensional Time-Series Data
Source: arXiv:2412.06870 source file (2024-12-09)
Supplement: Supplementary file 4 [file demo-particle-simulation.tex]

\begin{comment}

    \section{Particle Simulation}
    \label{sec:app-particle}
    
    
    
    
    \subsection{Setups}
    
    We trained the DMCF model~\citep{prantl-2022} having convolutions layers\footnote{The codebase for the training the DNN model is at \url{https://github.com/tum-pbs/DMCF/blob/main/models/cconv.py}}.
    The DNN model's training configuration is from the author on Github repository\footnote{\url{https://github.com/tum-pbs/DMCF/blob/96eb7fcdd5f5e3bdda5d02a7f97dfff86a036cfd/configs/WaterRamps.yml}}.
    The training data is from a ready-to-use dataset of the Waterramp scenario~\citep{sanchez-2020} that a particle simulator \emph{SPlish Splash} generates.
    The DNN model recursively predicts the next time step's particle blobs,
    i.e. the DNN model's input is all particles geo-coordinate at $t-1$, and the prediction output is the particles geo-coordinate at $t$.
    Because of this recursive prediction, prediction errors are accumulated over time and particle geo coordinate would become more and more dissimilar to the Splish-Splash simulation if the DNN model's prediction is not accurate.
    Figure~\ref{fig:demonstration-particle-sensor-256-particles-simulation} represents an example of the particle blobs from the Splish-Splash simulation and the DNN model at different time steps.
    The Splish-Splash output and the DNN model prediction apparently look dissimilar at the time step of $t=285$. 
    
    
    
    \begin{table}[h]
        \centering
        \begin{tabular}{c|c}
                \hline
                \includegraphics[width=0.44\textwidth]{images/demonstrations/particle-simulation/particles/snapshot-90.png} & 
                \includegraphics[width=0.44\textwidth]{images/demonstrations/particle-simulation/particles/snapshot-145.png} \\
                $\bucketIndex{1}, t=90$ &
                $\bucketIndex{2}, t=145$
                \\ \hline \hline
    
                \includegraphics[width=0.44\textwidth]{images/demonstrations/particle-simulation/particles/snapshot-285.png} &
                \includegraphics[width=0.44\textwidth]{images/demonstrations/particle-simulation/particles/snapshot-325.png} \\            
                $\bucketIndex{3}, t=285$ &           
                $\bucketIndex{4}, t=325$
                \\ \hline \hline
                
                \includegraphics[width=0.44\textwidth]{images/demonstrations/particle-simulation/particles/snapshot-440.png} &
                \includegraphics[width=0.44\textwidth]{images/demonstrations/particle-simulation/particles/snapshot-565.png} 
                \\
                $\bucketIndex{5}, t=440$ &
                $\bucketIndex{6}, t=565$ 
                \\ \hline
        \end{tabular}
        \caption{
            Particle blobs from a Splish-Splash simulation and the DNN model.
            blue particle blobs are from the Splish-Splash simulation,
            and green particle blobs are from the DNN model.
        }
        \label{fig:demonstration-particle-sensor-256-particles-simulation}
    \end{table}
    
    
    \subsection{Naive Approach: a naive L1 distance v.s. variable selection methods}
    \label{sec:demonstration-particle-naive-approach}
    
    A L1 distance (Absolute difference) is a naive but intuitive method for observing discrepancies.
    We compute the average L1 distance per observation sensor $d \in \{1,\threeDots,\Dim\}$ at each time bucket $b \in \{1,\threeDots\TotalBucketSize\}$,
    
    \begin{equation}
        \label{eq:average-l1-distance}
        {Avg\ L1}^d_b = \frac{1}{|\IntervalIndex{\bucket}|} \sum_{i=t_{b-1} + 1}^{t_b} |x^d_{i} - y^d_{i} |,
    \end{equation}
    where $x^d_{i}$ and $y^d_{i}$ are the counts of particles at a sensor $d$ from the Splish-Splash simulation and the DNN model, respectively, and $|\IntervalIndex{\bucket}|$ is the number of observations at the time bucket $\bucket$.
    Figure~\ref{fig:demonstration-particle-heatmaps-sensors} depicts comparisons of heatmaps by the average L1 distance and the variable selection methods.
    The heatmap by the averaged L1 distance, Figure~\ref{fig:demonstration-particle-heatmap-sensors-l1-diff}, shows that there are significant differences at buckets $\bucketIndex{2}$ and $\bucketIndex{3}$, which matches with our observation with the snapshots in Figure~\ref{fig:demonstration-particle-sensor-256-particles-simulation}.
    However, a drawback of the averaged L1 distance is that there are too many sensors representing discrepancies, and it would be time-consuming analysis work to confirm such sensors.
    Another drawback would be that the averaged L1 distance naturally focuses on sensors showing huge discrepancies;
    thus there is a possibility of missing discrepancies occurring by outliers which will be crucial information for the analysis of the DNN model's output.
    
    Figures~(\ref{fig:demonstration-particle-heatmap-sensors-wasserstein} - \ref{fig:demonstration-particle-heatmap-sensors-mmd-cv}) are heatmaps by the variable selection algorithms.
    Compared with the heatmap by the averaged L1 distance, the variable selection methods are able to dramatically reduce the number of variables (sensors).
    Therefore, analysts can focus on the selected sensors and investigate the discrepancies.
    Regarding discovering discrepancies that occurred by outliers, the MMD-based variable selection method successfully discovers such sensors, as we discuss Section~\ref{sec:demonstration-particle-result}.
    Table~\ref{fig:demonstration-particle-sensor-256-comparison-particle-vis-full} is a comparison of the selected variables in $\bucketIndex{2}, \bucketIndex{4}$.
    As we point out in Section~\ref{sec:demonstration-particle-result}, the DNN model prediction has unnatural water particles that seem to stick the ceil of the box at buckets $\bucketIndex{2}$ until $\bucketIndex{6}$.
    \codeName{MMD Selection} and \codeName{MMD CV} successfully discover such sensors, and the \codeName{Wasserstein-based} method does not.
    
    
    \begin{figure}
        \begin{subfigure}{\textwidth}
            \centering
            \includegraphics[scale=0.3]{images/demonstrations/particle-simulation/sensor_st/256/l1-difference-heatmap.png}
            \caption{Heatmaps by the average L1 distance}
            \label{fig:demonstration-particle-heatmap-sensors-l1-diff}
        \end{subfigure}
        \begin{subfigure}{0.33\textwidth}
            \centering
            \includegraphics[scale=0.3]{images/demonstrations/particle-simulation/sensor_st/256/variable-heatmaps-selected/heatmap-wasserstein_independence-.png}
            \caption{\codeName{Wasserstein-based}}
            \label{fig:demonstration-particle-heatmap-sensors-wasserstein}
        \end{subfigure}
        \begin{subfigure}{0.33\textwidth}
            \centering
            \includegraphics[scale=0.3]{images/demonstrations/particle-simulation/sensor_st/256/variable-heatmaps-selected/heatmap-interpretable_mmd-algorithm_one.png}
            \caption{\codeName{MMD selection}}
            \label{fig:demonstration-particle-heatmap-sensors-mmd-sel}
        \end{subfigure}
        \begin{subfigure}{0.33\textwidth}
            \centering
            \includegraphics[scale=0.3]{images/demonstrations/particle-simulation/sensor_st/256/variable-heatmaps-selected/heatmap-interpretable_mmd-cv_selection.png}
            \caption{\codeName{MMD CV}}
            \label{fig:demonstration-particle-heatmap-sensors-mmd-cv}
        \end{subfigure}
        \caption{
            Comparison of heatmaps.
            The horizontal and vertical axes are the indices of time buckets $\bucket$ and dimension (sensor-id).        
            \ref{fig:demonstration-particle-heatmap-sensors-l1-diff}: A heatmap of the average L1 distance per sensor at each time bucket.
            (\ref{fig:demonstration-particle-heatmap-sensors-wasserstein} - \ref{fig:demonstration-particle-heatmap-sensors-mmd-cv}) Heatmaps by the variable selection methods.
            The heatmap is based on weights $w \in \mathbb{R}^{D}$ per dimension at each time bucket.
            The weight is normalised in $[0.0, 1.0]$ per bucket $\bucket$ for ease of comparison.
            The heatmap shows only selected variables $\VariableSelectionHat$, and the rest of the values are $0.0$.
            When a p-value by the permutation test $\pValueTest{\bucket} > 0.05$, then all values at $\bucket$ are $0.0$.
            More descriptions are in Section~\ref{sec:demonstration-particle-naive-approach}.
            }
            \label{fig:demonstration-particle-heatmaps-sensors}
    \end{figure}
    
    
    
    
    
    \begin{table}[h]
        \centering
        \fontsize{6}{7}\selectfont
        \begin{tabular}{c|c|c}
                \hline
                &
                $\bucket{2}, t=145$ &
                $\bucket{6}, t=565$ \\
                \hline
                $\VariableSelectionHatIndex{\rm{Wass}}$ &
                \includegraphics[width=0.42\textwidth]{images/demonstrations/particle-simulation/sensor_st/256/represemtative_snapshots/wasserstein_baseline/wasserstein_independence--bucket1-145.png} & 
                \includegraphics[width=0.42\textwidth]{images/demonstrations/particle-simulation/sensor_st/256/represemtative_snapshots/wasserstein_baseline/wasserstein_independence--bucket5-565.png} \\
                \hline
                $\VariableSelectionHatIndex{\rm MMD\ Sel}$ &
                \includegraphics[width=0.42\textwidth]{images/demonstrations/particle-simulation/sensor_st/256/represemtative_snapshots/mmd_model_selection/interpretable_mmd-algorithm_one-bucket1-145.png} & 
                \includegraphics[width=0.42\textwidth]{images/demonstrations/particle-simulation/sensor_st/256/represemtative_snapshots/mmd_model_selection/interpretable_mmd-algorithm_one-bucket5-565.png} \\
                \hline
                
                $\VariableSelectionHatIndex{\rm MMD\ CV}$ &
                \includegraphics[width=0.42\textwidth]{images/demonstrations/particle-simulation/sensor_st/256/represemtative_snapshots/mmd_cv_aggregation/interpretable_mmd-cv_selection-bucket1-145.png} & 
                \includegraphics[width=0.42\textwidth]{images/demonstrations/particle-simulation/sensor_st/256/represemtative_snapshots/mmd_cv_aggregation/interpretable_mmd-cv_selection-bucket5-565.png} \\
        \hline
        \end{tabular}
        \caption{
            Comparison of three variable selection methods. 
            In each table element,
            the blue particles (left) are from the Splish-Splash simulator,
            and the green particles (right) are from the DMCF model.
            The red highlighting boxes are selected sensors by the variable selection method. 
            We select and represent representative time steps at each bucket $\bucket$.
            We do not show the red highlighting box when p-value > 0.05. 
            More descriptions are in Section~\ref{sec:demonstration-particle-result}.
        }
        \label{fig:demonstration-particle-sensor-256-comparison-particle-vis-full}
    \end{table}
        
    
    
    
    \subsection{Variable Selection for particle trajectories}
    \label{sec:demonstration-particle-variable-selection-trajectory}
    
    We clearly see that the DNN model's prediction output has discrepancies compared with the Splish-Splash simulation.
    To comprehend and explain the reasons more, one may be interested in discrepancies in the directions of water particle trajectories.
    Once discrepancies in water particles are identified, it would be useful for improving the DNN model's prediction output.
    For example, XAI (Explainable AI) methods can be applied to identify relationships between the DNN model's input features and detected simulation agents.
    We apply the variable selection and permutation test for trajectories, which we introduce in Section~\ref{sec:appendix-variable-selection-trajectory}.
    
    Two time-series $X, Y$ consist of $\mathbb{R}^{A \times \TimeN \times C}$ as we describe in Section~\ref{sec:demonstration-particle-setup}, where $X$ is from the SPlisHSPlasH simulator, and $Y$ is from the DNN model.
    Following the data representation in Section~\ref{sec:appendix-variable-selection-trajectory} that we convert these time-series to $\mathbb{R}^{A \times (\TimeN-1) \times C}$ by subtracting the geo-coordinates between $t-1$ and $t$ for all particles.
    All configurations of the time-slicing algorithm and variable selection methods are the same as Section~\ref{sec:demonstration-particle-setup}.
    
    Figure~\ref{fig:demonstration-particle-sensor-256-p-values-with-trajectory} visualises the p-values at each bucket.
    Although the plot in the left \ref{fig:demonstration-particle-sensor-256-p-values-replot} is the same as the plot in Figure~\ref{fig:demonstration-particle-sensor-256-p-values}, we plot it again for comparison.
    Figure~\ref{fig:demonstration-particle-sensor-256-p-values-trajectory} is the p-value sequence by the water particle trajectories.
    At the 1st bucket, $\bucketIndex{1}$, two MMD-based methods accept $H_0$ and the Wasserstein-based method rejects $H_0$.
    From the 2nd bucket $\bucketIndex{2}$ until the end, all methods reject $H_0$.
    This result implies that the DNN model's prediction output would behave relatively similar to the output of the Splish-Splash simulations at the 1st bucket (until the 100th time step), and then the trajectory behaves differently after the 100th time step.
    Looking at the snapshots in Figure~\ref{fig:demonstration-particle-sensor-256-particles-simulation}, in the 2nd bucket $\bucketIndex{2}$, blue water particles (SPlish-SPlash) start to form a certain line in the centre of the box, 
    whereas green particles (DNN model) fail to form such a line, rather say, spread out.
    Considering that the particles in 2nd bucket are after actions that water particles rebound at the floor of the box, the discrepancies of green particles are due to either emulating rebounding actions or emulating collision between particles.
    
    Figure~\ref{fig:demonstration-particle-sensor-256-p-values-trajectory-snapshots} illustrates variable selection results at $t=145$ in the 2nd bucket $\bucketIndex{2}$.
    Particles detected by all variable selection methods are located far from each other between the blue and green particles, which explains the reason that this DNN's model prediction looks dissimilar from the SPlish-SPlash simulation illustrated in Figure~\ref{fig:demonstration-particle-sensor-256-particles-simulation}.
    Compared to the selection result of \codeName{wasserstein-based}, the MMD-based methods notably detect particles that exit at totally dissimilar positions.
    This result illustrates that DNN model prediction has significant errors already at $t=145$ which is accumulated through the recursive prediction. 
    
    
    \begin{figure}
        \begin{subfigure}{0.45\textwidth}
            \centering
            \includegraphics[scale=0.4]{images/demonstrations/particle-simulation/sensor_st/256/p-value-sequence.png}
            \caption{Observation sensors data}
            \label{fig:demonstration-particle-sensor-256-p-values-replot}
        \end{subfigure}
        \begin{subfigure}{0.45\textwidth}
            \centering
            \includegraphics[scale=0.4]{images/demonstrations/particle-simulation/trajectory-st/p-value-sequence.png}
            \caption{Water particles trajectories}
            \label{fig:demonstration-particle-sensor-256-p-values-trajectory}
        \end{subfigure}
        \caption{
            A comparison of p-value sequences of permutations tests by the observation sensors data (\ref{fig:demonstration-particle-sensor-256-p-values}) and the directions of trajectory data (\ref{fig:demonstration-particle-sensor-256-p-values-trajectory}).
            Figure~\ref{fig:demonstration-particle-sensor-256-p-values-replot} is the same plot as Figure~\ref{fig:demonstration-particle-sensor-256-p-values}.
            Figure~\ref{fig:demonstration-particle-sensor-256-p-values-trajectory} is the p-value sequence by the water particle trajectories.
            The red dot lines are at $p=0.05$ for rejecting $H_0$.
            More descriptions are in Section~\ref{sec:demonstration-particle-variable-selection-trajectory}.
        }
        \label{fig:demonstration-particle-sensor-256-p-values-with-trajectory}
    \end{figure}
    
    
    \begin{figure}
        \begin{subfigure}{0.45\textwidth}
            \centering
            \includegraphics[scale=0.4]{images/demonstrations/particle-simulation/trajectory-st/represemtative_snapshots/wasserstein_baseline/wasserstein_independence--bucket1-145.png}
            \caption{\codeName{Wasserstein-based}}
        \end{subfigure}
        \begin{subfigure}{0.45\textwidth}
            \centering
            \includegraphics[scale=0.4]{images/demonstrations/particle-simulation/trajectory-st/represemtative_snapshots/mmd_model_selection/interpretable_mmd-algorithm_one-bucket1-145.png}
            \caption{\codeName{MMD selection}}
        \end{subfigure}
        \begin{subfigure}{0.45\textwidth}
            \centering
            \includegraphics[scale=0.4]{images/demonstrations/particle-simulation/trajectory-st/represemtative_snapshots/mmd_cv_aggregation/interpretable_mmd-cv_selection-bucket1-145.png}
            \caption{\codeName{MMD CV}}
        \end{subfigure}
        \caption{
            Comparison of three variable selection methods for water particles at the 2nd bucket $\bucketIndex{2}$.
            The blue particles (left) are from the Splish-Splash simulator,
            and the green particles (right) are from the DMCF model.
            Variable selection methods detect red-coloured particles having the same particle-ids.
            More descriptions are in Section~\ref{sec:demonstration-particle-variable-selection-trajectory}.
        }
        \label{fig:demonstration-particle-sensor-256-p-values-trajectory-snapshots}
    \end{figure}
    
    \end{comment}
    
    
    
